# Supplementary material for: Unsupervised Deep Manifold Attributed Graph Embedding
Source: arXiv:2104.13048 source file (2021-04-27)
Supplement: Supplementary file 1 [file appendix_changing_nv.tex]

\section{Changing Hyperparameter $\nu$}

The hyperparameter $\nu_{latent}$ is the degree of freedom of the t-distribution in the latent space and controls the sharpness of the distribution. If $\nu_{latent}$ is small, a sharper t-distribution will drive the nearest neighbors in the latent space to cluster together to form clusters. If $\nu_{latent}$ is larger, a flatter t-distribution will induce the nearest neighbor points in the latent space to loosely open up to a manifold. The experiments results of changing $\nu_{latent}$ is shown in the Fig.~\ref{fig:a_vis_changing_nu}. 

All other hyperparameter settings are the same as for the node clustering, linkage prediction task, and for each dataset, we pick the range of variation that is appropriate to demonstrate.The results for all datasets show that smaller $\nu_{latent}$ makes the nodes more compact among themselves, which means more local information is discarded, although this has some benefits for the clustering task. On the contrary, increasing $\nu_{latent}$ makes the local details amplified, but destroys the global structure of the data, and the points of different clusters are diffused together.

\begin{figure}[!htb]
    \centering
    \includegraphics[width=5in]{./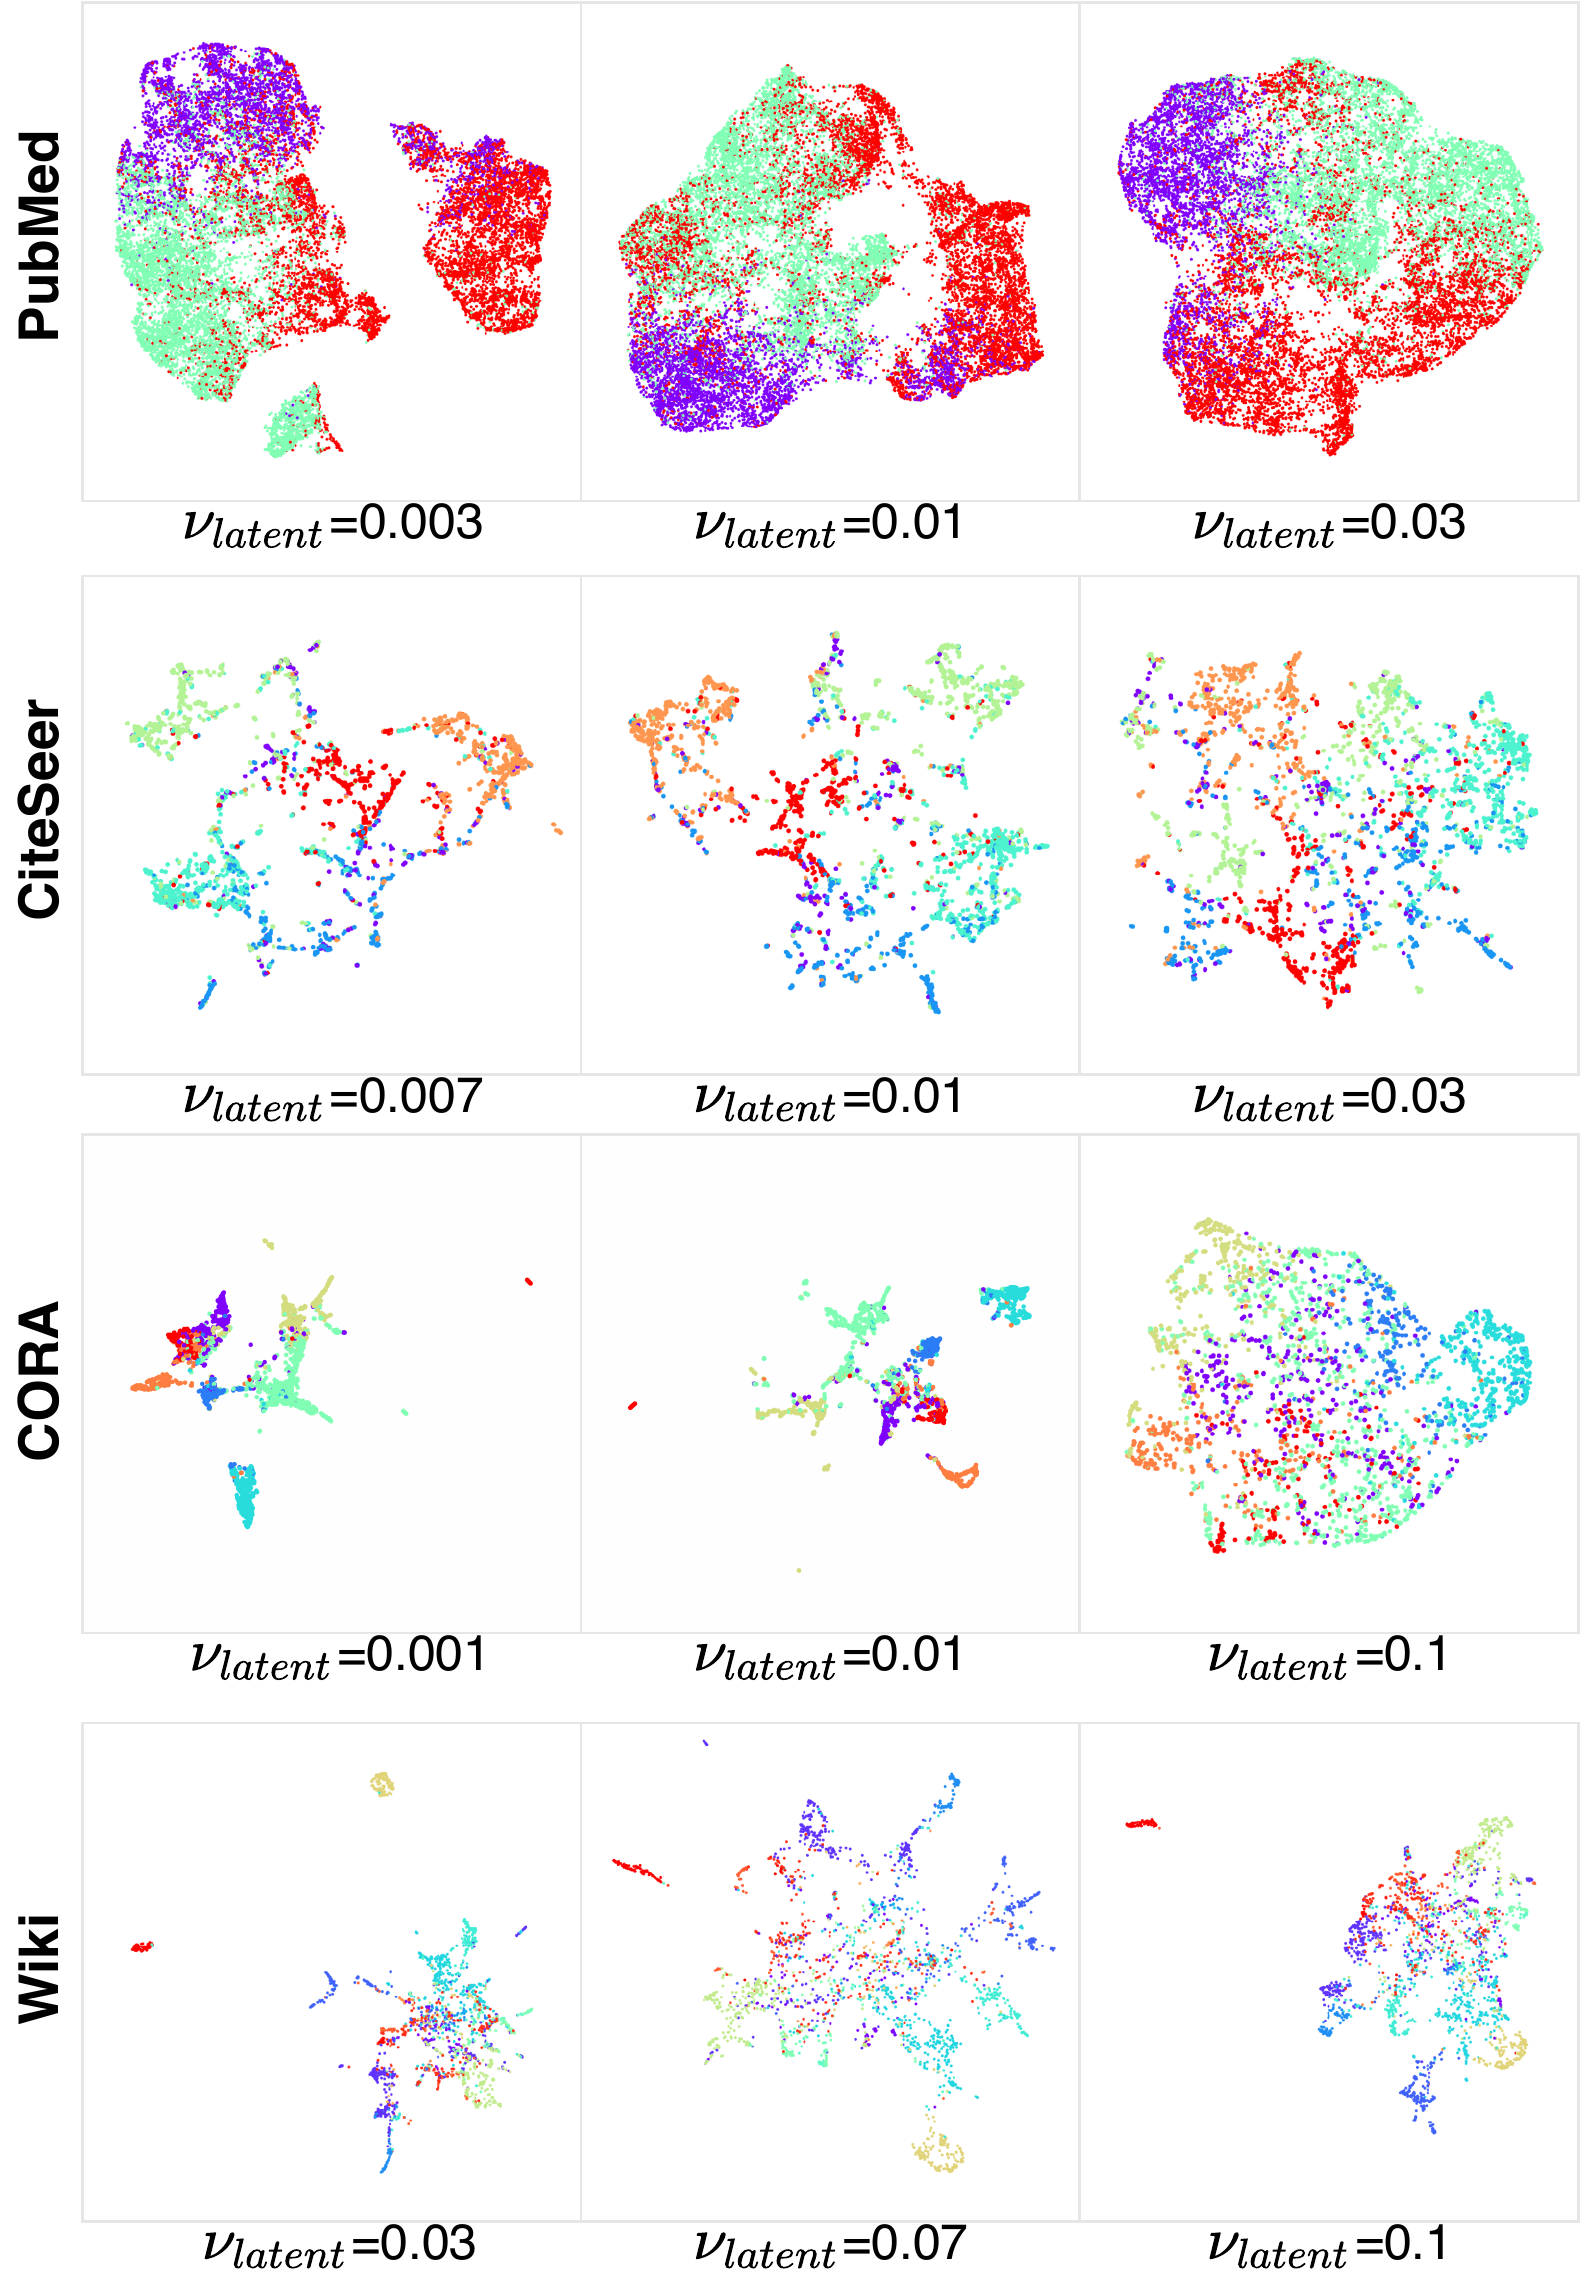}
    \caption{2D visualization of different embeding on varying the latent space t-distribution degrees of freedom  $\nu_{latent}$. }
    \label{fig:a_vis_changing_nu}
  \end{figure}
