# Supplementary material for: Unsupervised Deep Manifold Attributed Graph Embedding
Source: arXiv:2104.13048 source file (2021-04-27)
Supplement: Supplementary file 2 [file appendix_pseudoCode.tex]

\section{Pseudo code and of our algorithm}
The pseudo code of our method to generate graph node embedding is as follows.
{
    \large
    \begin{algorithm}[ht]
        \caption{G-ELIS}
        \SetAlgoLined
        \textbf{ Input }: \\
        \ \ \ \ \ \ \ \ \ \ \ \ \ \ Graph : $G=({V}, \mathcal{E}, {X})$, \\
        \ \ \ \ \ \ \ \ \ \ \ \ \ \ Learning rate : $l_r$, \\
        \ \ \ \ \ \ \ \ \ \ \ \ \ \ Epochs : $E_p$,\\
        \ \ \ \ \ \ \ \ \ \ \ \ \ \ Batch szie : $B_s$,\\
        \ \ \ \ \ \ \ \ \ \ \ \ \ \ Network structure : $N_S$,\\
        \ \ \ \ \ \ \ \ \ \ \ \ \ \ Weight hyperparameter : $\alpha$,\\
        \ \ \ \ \ \ \ \ \ \ \ \ \ \ Degree of freedom : $\nu_{latent}$,\\
        \ \ \ \ \ \ \ \ \ \ \ \ \ \ Neighbor prior distribution parameter : $Q_p$\\
        \textbf{ Output }: \\
        \ \ \ \ \ \ \ \ \ \ \ \ \ \ Graph Embedding : $Z$, \\
        \ \\ 
        \textcolor{green!55!blue}{\# Initialization}\\ 
        Calculate $D^{G_X}$ and $D^{\bar G_X}$ with equ.~(\ref{equ:D_X^G})  \\
        Calculate $\sigma_{input}$ use $Q_p$, $\nu_{input}=100$ and $D^{G_X}$ as input with equ.~(\ref{equ:bin_search}) \\
        Calculate $P^{G_X}_{i|j}$ and $P^{\bar G_X}_{i|j}$ use $\sigma_{input}$ and $D^{G_X}$ as input  with equ.~(\ref{equ:P_ij^G}) - (\ref{equ:bin_search})\\
        Calculate $P^{G_X}$ and $P^{\bar G_X}$ with equ.~(\ref{equ:simi})\\
        Initialize the neural network $\phi(\ \ \cdot\ \ |W)$ with Network structure $N_S$\\
        \ \\
         \textcolor{green!55!blue}{\# epcoh loop}\\ 
        \While{$i=0$; $i<E_p$; $i$++}{
            \ \\    
            \textcolor{green!55!blue}{\# batch loop}\\ 
            \While{$b=0$; $b<[ |V| /B_s]$; $b$++}{
            % $\nu \longleftarrow \nu_{List}[i]$ \\
            Graph structure augmentation with equ.~(\ref{equ:hatE}), $A^*\longleftarrow A_{ug}(A)$\\
            Network forward propagation with equ.~(\ref{equ:phi}), $Z \longleftarrow \phi(X, A^*|W)$\\
            Calculate $D^{\bar G_Z}$ use $G_Z(V, \bar E, Z)$ as input with equ.~(\ref{equ:D_X^G}).\\
            Calculate $Q^{\bar G_Z}$ with equ.~(\ref{equ:P_ij^G}) and (\ref{equ:simi})\\
            Calculate the loss with equ.~(\ref{equ:L^G}) and equ.~(\ref{equ:LmathcalG}), $ L\longleftarrow L(  P^{\bar G_X}, Q^{\bar G_Z} ) + \alpha L( P^{G_X}, Q^{\bar G_Z} )$
            \\
            Update parameters: $W \longleftarrow W - l_r \frac{ \partial \mathcal{L} }{\partial W_{Enc}}$
            }
        }
        Get the final embedding result, $Z \longleftarrow \phi(X, A|W)$
    \end{algorithm}

}    

We analyze the time complexity of the algorithm in two parts: initialization and iterative learning. 
The time consumption in the initialization part is mainly in computing the point pair distances and computing the shortest paths. The complexity of computing the point pair distance is $O(|V|^2)$ but it can be easily hardware accelerated. Using the traditional Dijkstra algorithm to solve the shortest path, the time complexity is $O(|E|+|V| \log |V|)$, where $|E|$ is the number of nodes and $|V|$ is the number of edges.

The operation with the highest time complexity of the training process is the calculation of the embedded point-to-point distance. However, due to the use of minibatch, the time complexity is $O(B_s)$.
